# Supplementary material for: SPOT: Knowledge-Enhanced Language Representations for Information Extraction
Source: arXiv:2208.09625 source file (2022-10-24)
Supplement: Supplementary file 1 [file 6_appendix.tex]

\section{Appendix}
\vspace*{0.5cm}

\subsection{Implementation Details and Hyperparameters}
\label{sec:details_hyper}
  We use a single GPU for all fine-tuning on downstream information extraction tasks.

For all information extraction tasks, we use the Adam optimizer and select the best learning rate from \{1e-5, 2e-5, 5e-5\}, the best warmup steps from \{$0, 300, 1000$\} and the best weight decay from \{$0.01$, 1e-5\}. We adopt linear learning rate decay strategy and gradient is clipped to $5$ for all experiments. The dropout ratio is $0.1$ for language model and $0.3$ for task-specific layers. The batch size is $16$ for joint learning entities and relationships, entity typing, named entity extraction and $32$ for relation extraction task. We adopt early stop by using the best model on development set and test on test set.

\subsection{Ablation Study Experiments}
\label{app:ablation}
In the ablation study, we set the same hyper-parameters for all experiments. Specifically, the batch size is $16$ and we use Adam optimizer with learning rate 2e-5 and linear learning rate decay. All gradients are clipped to $5$ and warm up steps are $300$. We adopt early stop by using the best model on development set and test on test set. When we use two kinds of encoder, we concatenate the two output of encoders and feed the concatenation to a linear classifier.
